# Supplementary material for: A Multi-Objective Portfolio of Portfolios Problem with Qualitative Performance Assessments
Source: arXiv:2503.02373 source file (2025-03-04)
Supplement: Supplementary file 1 [file Appendix.tex]

%%Both these tables to be inserted in the Appendix%%
\begin{table}
\centering\caption{ Qualitative thresholds for each researcher on the four criteria}\label{Tab:vhjsesempio}
\makebox[\linewidth]{
\begin{tabu}{|c|c|c||c|c||c|c||c|c|}
\hline
\ \multirow{2}{*}{$v_{hjs}$}  &  \multicolumn{2}{c||} {$g_1$} & \multicolumn{2}{c||}  {$g_2$} &   \multicolumn{2}{c|} {$g_3$} &   \multicolumn{2}{c|} {$g_4$}  \\
       \cline{2-9}
     & $l_1$ & $l_2$ & $l_1$ & $l_2$ & $l_1$ & $l_2$& $l_1$ & $l_2$   \\
     \hline
$e_1	$&	0&	0&	1&	1&	1&	1&	0&	0\\
$e_2	$&	1&	0&	1&	1&	1&	0&	1&	0\\
$e_3	$&	1&	1&	1&	0&	1&	1&	1&	1\\
$e_4	$&	1&	0&	1&	1&	1&	1&	1&	1\\
$e_5	$&	1&	0&	1&	1&	1&	1&	1&	0\\
$e_6	$&	1&	1&	1&	1&	1&	0&	1&	0\\
$e_7	$&	1&	0&	1&	1&	0&	0&	0&	0\\
$e_8	$&	1&	0&	1&	1&	1&	1&	1&	1\\
\hline
\end{tabu}
}
\end{table}%%

\begin{table}
\centering\caption{ Minimal number of researchers to be assigned to each project.}\label{Tab:MinimalNumberProjects}
\makebox[\linewidth]{
\begin{tabu}{|c|c|c||c|c||c|c||c|c|}
\hline
\ \multirow{2}{*}{$w_{kjs}$}   &  \multicolumn{2}{c||} {$P_1$} & \multicolumn{2}{c||}  {$P_2$} &   \multicolumn{2}{c|} {$P_3$} &   \multicolumn{2}{c|} {$P_4$}  \\
       \cline{2-9}
      & $l_1$ & $l_2$ & $l_1$ & $l_2$ & $l_1$ & $l_2$ & $l_1$ & $l_2$  \\
      \hline
$g_1$ & 3 & 1 & 4 & 2 & 3 & 2 & 4 & 1 \\
$g_2$ & 2 & 1 & 3 & 2 & 2 & 1 & 1 & 1 \\
$g_3$ & 2 & 1 & 3 & 0 & 4 & 2 & 2 & 1 \\ 
$g_4$ & 2 & 0 & 4 & 1 & 1 & 1 & 0 & 0\\     
\hline
\end{tabu}
}
\end{table}
